# Supplementary material for: Ollivier-Ricci Curvature of Riemannian Manifolds and Directed Graphs with Applications to Graph Neural Networks
Source: arXiv:2604.14211 source file (2026-08-24)
Supplement: Supplementary file 1 [file appendix.tex]

\chapter{}
\section*{Review of Classical Ricci Curvature and Selected Results}

\begin{itemize}
  \item A Riemannian $n$-manifold with metric $g$ is denoted $\left(M^{n}, g\right)$.
  \item $\frac{\partial}{\partial x_{i}}$ on $M$ denotes the push-forward of $\frac{\partial}{\partial x_{i}}$ under some chart $\varphi: U \rightarrow M$ on $M$, where $U \subseteq \mathbb{R}^{n}$.
  \item $D_{p} f$ for $f: M \rightarrow N$ denotes the derivative $D_{p} f: T_{p} M \rightarrow T_{f(p)} N$.
  
  \item $\mathfrak{X}(M)$ denotes the collection of all smooth vector fields on $M$.
\end{itemize}

\begin{definition}
A map $T: \underbrace{\mathfrak{X}(M) \times \mathfrak{X}(M) \times \cdots \times \mathfrak{X}(M)}_{r \text { times }} \rightarrow C^{\infty}(M)$

is an $r$-tensor if for all $f \in C^{\infty}(M), X_{1}, \ldots, X_{r} \in \mathfrak{X}(m)$, 
$$
T\left(X_{1}, \ldots, f X_{j}, \ldots, X_{r}\right)=f T\left(X_{1}, \ldots, X_{r}\right) .
$$
    
\end{definition}

\begin{definition} \cite{PetersenPeter2006Rg}
Let $(M, g)$ be a Riemannian manifold and $\nabla$ the Riemannian connection. Let $X, Y, Z \in  $

We define the \textit{Riemannian curvature operator} for $X, Y, Z $ as a $(1,3)$-tensor as follows:
$$
\begin{aligned}
R(X, Y) Z & =\nabla_{X, Y}^{2} Z-\nabla_{Y, X}^{2} Z \\
& =\nabla_{X} \nabla_{Y} Z-\nabla_{Y} \nabla_{X}-\nabla_{[X, Y]} Z \\
& =\left[\nabla_{X}, \nabla_{Y}\right] Z-\nabla_{[X, Y]} Z
\end{aligned}
$$

We will prove that indeed the Riemannian curvature tensor is a tensor. It is sufficient to show that $R$ is tensorial in $Z$ given that the second covariant derivatives are tensorial in $X$ and $Y$.
\end{definition}
\begin{lemma}
$R(X, Y) (f Z) = f R(X, Y) Z $
\end{lemma}
\begin{proof} Observe that
$$
\begin{aligned}
\nabla_{X}\left(\nabla_{Y}(f Z)\right) & =\nabla_{X}\left(Y(f) Z+f \nabla_{Y} Z\right) \\
& =X(Y(f)) Z+Y(f) \nabla_{X} Z+X(f) \nabla_{Y} Z+f \nabla_{X} \nabla_{Y} Z \\
\nabla_{Y}\left(\nabla_{X}(f Z)\right) & =  
\nabla_{Y}\left(X(f) Z+f \nabla_{X} Z\right) 
\\
&= Y(X(f)) Z+X(f) \nabla_{Y} Z+Y(f) \nabla_{X} Z+f \nabla_{Y} \nabla_{X} Z 
\end{aligned}
$$
From this we can obtain,
$$
\begin{aligned}
\nabla_{X}\left(\nabla_{Y}(f Z)\right)-\nabla_{Y}\left(\nabla_{X}(f Z)\right) & =X(Y(f)) Z-Y(X(f)) Z+f \nabla_{X} \nabla_{Y} Z-f \nabla_{Y} \nabla_{X} Z \\
& =[X, Y](f) \cdot Z+f \nabla_{X} \nabla_{Y} Z-f \nabla_{Y} \nabla_{X} Z .
\end{aligned}
$$
Furthermore we have, 
$$
\nabla_{[X, Y]}(f Z)=[X, Y](f)+f \nabla_{[X, Y]}(Z) .
$$
It follows that
$$
\begin{aligned}
R(X, Y)(f Z) &= f \nabla_{X} \nabla_{Y} Z-f \nabla_{Y} \nabla_{X} Z-f \nabla_{[X, Y]}(Z) \\ &= f R(X, Y)(Z) 
\end{aligned}
$$
\end{proof}

For any coordinate tangent basis, the curvature tensor can be written in terms of it components as follows: 

$$
R=R_{i k j}^{l} d x^{i} \otimes d x^{k} \otimes d x^{j} \otimes \partial_{l}
$$

In a local coordinate system $(x^1, x^2,...,x^n)$ then we can choose the coordinate basis vectors $\frac{\partial}{\partial x^i} = \partial_i$. The curvature tensor can be expressed in terms of these basis vectors, 
\[
R\left( \frac{\partial}{\partial x^i}, \frac{\partial}{\partial x^j} \right) \frac{\partial}{\partial x^k} = R^l_{\ ijk} \frac{\partial}{\partial x^l}.
\]

where the components \( R^l_{\ ijk} \) are the coefficients of the Riemann curvature tensor in this basis and the upper index $l$ represents the output instead of the curvature tensor. Recall that the curvature tensor tensor $R(X,Y)Z$ takes in vector fields $X,Y,Z$ and outputs a new vector field that measures how much the vector field $Z$ changes after being parallel transported around the parallelogram formed by the vector fields $X$ and $Y$.

The symmetric metric tensor $g_{pq}$ that defines distances and angles, for example, in a space can be used to raise and lower the indices of tensors like the curvature tensor. For example, $g_{qp}$ represents the component of the metric tensor at index positions $q$ and $p$, or in other words how much the coordinate basis vectors $\partial_p$ and $\partial_q$ are related in terms of the metric-defined inner product. Take $ R^l_{\ ijk}$. Then $g_{lp}$ contracts the index $p$ to lower the upper index $l$:
\[
R_{ijkl} = g_{lp} R^p_{\ ijk}.
\]
and therefore $g$ contracts the curvature tensor from $(1,3)$ type to a $(0,4)$ type tensor. Going back to our original notation, therefore, we have:
$$
R(X, Y, Z, W)=g(R(X, Y) Z, W)
$$

The curvature of a Riemannian manifold $M$ can be understood as a measure $R(X, Y) Z$ of the extent to which the operator $(X, Y) \mapsto \nabla_{X} \nabla_{Y} Z$ is symmetric, where $\nabla$ is a connection on $M$ and where $X, Y, Z$ are vector fields, with fixed $Z$. The operator $R(X, Y) Z$ is $C^{\infty}(M)$ linear in all of its three arguments, so for all $p \in M$, we have the following trillinear map:
$$
R_{p}: T_{p} M \times T_{p} M \times T_{p} M \longrightarrow T_{p} M
$$

Intuitively we can interpret the Riemann tensor as capturing how parallel transport fails to close around small loops. A manifold is considered flat, or have zero curvature, if its Riemann curvature tensor vanishes. 

\begin{proposition} \cite{PetersenPeter2006Rg}
The curvature tensor $R$ satisfies the following symmetry properties. 
\begin{enumerate} 
    \item[(a)] $R_{i k j l}+R_{k i j l}=0$ 
    \item[(b)] $R_{i k j l}+R_{k j i l}+R_{j i k l}=0$ 
    \item[(c)]  $R_{i k j l}+R_{i k l j}=0$ 
    \item[(d)] $R_{i k j l}=R_{j l i k}$.
\end{enumerate}
\end{proposition}
\begin{proof} (a) $R_{i k j l}+R_{k i j l}=0$ follows from the definition of curvature. Recall that
$R(X, Y) Z = 
\nabla_{X} \nabla_{Y} Z-\nabla_{Y} \nabla_{X}-\nabla_{[X, Y]} Z
$. By Leibniz rule, $R(X,Y)Z = -R(Y,X)Z$. Therefore, it is obvious that if $R_{ijk}^l = -R_{kij}^l$ then $R_{ijkl} = -R_{kijl} $.
\end{proof}
\begin{proof} (b) This is called the first Bianchi identity. By definition of the curvature tensor we have:
$$
R_{ikjl} = g(R(\partial_i, \partial_k) \partial_j, \partial_l) = g(\nabla_k \nabla_j \partial_i - \nabla_j \nabla_k \partial_i, \partial_l)
$$
Which we can rearrange as: 
$$
R_{ikjl}  = g\left(\nabla_{k}\left(\nabla_{i} \partial_{j}-\nabla_{j} \partial_{i}\right), \partial_{l}\right) 
$$

Indices are arbitrary, so we similarly obtain:
   \[
   R_{kjil} = g\left(\nabla_{j}\left(\nabla_{k} \partial_{i}-\nabla_{i} \partial_{k}\right), \partial_{l}\right)
   \]
   \[
   R_{jikl} = g\left(\nabla_{i}\left(\nabla_{j} \partial_{k}-\nabla_{k} \partial_{j}\right), \partial_{l}\right)
   \]
   
$$
\begin{aligned}
\implies R_{i k j l}+R_{k j i l}+R_{j i k l}
= & g\left(\nabla_{k}\left(\nabla_{i} \partial_{j}-\nabla_{j} \partial_{i}\right), \partial_{l}\right) \\
& +g\left(\nabla_{j}\left(\nabla_{k} \partial_{i}-\nabla_{i} \partial_{k}\right), \partial_{l}\right) \\
& + g\left(\nabla_{i}\left(\nabla_{j} \partial_{k}-\nabla_{k} \partial_{j}\right), \partial_{l}\right) = 0
\end{aligned}
$$
b the three terms cancel out because we assume the connection is torsion-free,  $[\partial_i, \partial_j] = 0$ and therefore $\nabla_{i} \partial_{j}-\nabla_{j} \partial_{i} \rightarrow 0$  and analogous inner terms of alternate indices.   
\end{proof} 
\begin{proof}  (c) Recall that
$$ R_{j i k l} + R_{j i l k} = g\left(\nabla_i \nabla_j \partial_k - \nabla_j \nabla_i \partial_k, \partial_l \right) + g\left(\nabla_i \nabla_j \partial_l - \nabla_j \nabla_i \partial_l, \partial_k \right)
$$
By bilinearity of $g$, 
$$
g(\nabla_i \nabla_j \partial_k - \nabla_j \nabla_i \partial_k, \partial_l) =
g(\nabla_i \nabla_j \partial_k, \partial_l) - g(\nabla_j \nabla_i \partial_k, \partial_l)
$$

Recall that by metric compatibility and Leibniz rule, 
$$
g(\nabla_i \nabla_j \partial_k, \partial_l) = \partial_i g(\nabla_j \partial_k, \partial_l) - g(\nabla_j \partial_k, \nabla_i \partial_l)
$$
Therefore, 
$$
\begin{aligned}
R_{j i k l} + R_{j i l k} &= g\left(\nabla_{i} \nabla_{j} \partial_{k}, \partial_{l}\right) + g\left(\nabla_{i} \partial_{k}, \nabla_{j} \partial_{l}\right) + g\left(\nabla_{j} \partial_{k}, \nabla_{i} \partial_{l}\right) + g\left(\partial_{k}, \nabla_{i} \nabla_{j} \partial_{l}\right) \\
&\quad - g\left(\nabla_{j} \nabla_{i} \partial_{k}, \partial_{l}\right) - g\left(\nabla_{j} \partial_{k}, \nabla_{i} \partial_{l}\right) - g\left(\nabla_{i} \partial_{k}, \nabla_{j} \partial_{l}\right) - g\left(\partial_{k}, \nabla_{j} \nabla_{i} \partial_{l}\right) \\
&= \partial_{i}\left(g\left(\nabla_{j} \partial_{k}, \partial_{l}\right) + g\left(\partial_{k}, \nabla_{j} \partial_{l}\right)\right) 
- \partial_{j}\left(g\left(\nabla_{i} \partial_{k}, \partial_{l}\right) + g\left(\partial_{k}, \nabla_{i} \partial_{l}\right)\right) \\
&= \partial_{i} \partial_{j} g_{k l} - \partial_{j} \partial_{i} g_{k l} \\
&= 0.
\end{aligned}
$$
The second to last line is due to the fact that the metric compatability condition implies that \\ $g\left(\nabla_{j} \partial_{k}, \partial_{l}\right) + g\left(\partial_{k}, \nabla_{j} \partial_{l}\right) = \partial_i g_{kl}$. The last line is due to the fact that the partial derivatives commute such that $\partial_{i} \partial_{j} g_{k l} = \partial_{j} \partial_{i} g_{k l}$.

\end{proof}
\begin{proof} (d)
We prove this by interchangeably using properties (a),(b), and (c):
\begin{align*}
R_{i k j l}  &= -R_{k j i l}-R_{j i k l}  \\
&= R_{k j l i}+R_{j i l k}  
- R_{j l k i}-R_{l k j i}-R_{i l j k}-R_{l j i k} \\
&= 2 R_{j l i k}+R_{l k i j}+R_{i l k j} \\
&=2 R_{j l i k}-R_{k i l j} \\
&= 2 R_{j l i k}-R_{i k j l} \\
&\implies R_{i k j l}=R_{j l i k}
\end{align*}
\end{proof}
We can use these symmetry and anti-symmetry properties to easily understand Riemannian curvature on 1-dimensional and 2-dimensional manifolds:
\begin{example} Let $M$ be a $1-$dimensional manifold such that at any point $p$, the tangent space $T_p M$ has dimension $1$ with $e_1$ as a basis vector. Therefore any three vectors inputted into the curvature tensor will be linearly dependent. Recall by the ant-symmetry properties proved above that $R(e_1, e_1, e_1) = -R(e_1, e_1, e_1)$, requiring that $R(e_1, e_1, e_1) = 0$. Thus the curvature is always zero on $1-$dimensional manifold, which intuitively makes sense because Riemmanian curvature is an \textit{intrinsic} curvature notion. A 1-dimensional line or curve cannot be intrinsically bent or curved at any point, which is not to be confused with extrinsic curvature of a line that is possible once embedded in a higher dimensional space. 
\end{example}
\begin{example} Let $M$ be a $2-$dimensional manifold such that at any point $p$, the tangent space $T_p M$ has dimension 2 with $e_1, e_2$ as a basis vectors. We can only have indices  $i = 1$ and $j = 2$ in this case. Consider the possible components that could satisfy the curvature tensor property of anti-symmetry under the swapping of the first two components and anti-symmetric under the swapping of the last two components. Consider if $R_{1112}$ was a component. Then, $R_{1112} = - R_{1112} \implies R_{1112} = 0$ and that component vanishes. 
\end{example}

\begin{example} Let $M$ be an n-dimensional manifold. We can generalize the previous examples above to $n$ dimensions. If the tangent space $T_p M$ at any point $p$ on $M$ has basis vectors $\{e_1, e_2,...,e_n\}$ then for all arbitrary basis vectors $\{e_\alpha, e_\beta, e_\sigma, e_\gamma\} $ then $R_{\alpha\Beta \sigma \gamma}$ will depend solely on the $2-$dimensional plane generated by $e_\alpha$ and $e_\beta$, as well as the $2-$dimensional plane generated by $e_\sigma$ and $e_\beta$. 
\end{example}

As a consequence of the previous example, we will discuss now introduce sectional curvature. 
\begin{definition} Fix $x \in M, P \subseteq T_{p} M$ a 2-plane where $e_{1}, e_{2}$ is an orthonormal basis for $P$
. Then the \textit{sectional curvature} of $P$ at $x$ is
$$
K_{x}(P):=R \left(e_{1}, e_{2}, e_{2}, e_{1}\right),
$$
\end{definition}
\begin{lemma}
Suppose $R_{1}, R_{2}: T_{x} M \times T_{x} M \times T_{x} M \times T_{x} M \rightarrow \mathbb{R}$ are both multilinear maps endowed with the same symmetries properties as curvature tensor $R$ from Proposition 4.1.4. If $K_{1}(P)=K_{2}(P)$ for all 2-planes $P \subseteq T_{x} M$, then $R_{1}=R_{2}$. In other words, section curvature determines $R$.
\end{lemma}
\begin{corollary}
Let $\left(M^{2}, g\right)$ be a surface, such that the sole 2-plane is $K_{x}\left(T_{x} M\right)=: K(x)$. Then,
$$
\mathcal{R}(X, Y, Z, W)=K(x)(\langle X, W\rangle\langle Y, Z\rangle-\langle X, Z\rangle\langle Y, W\rangle)
$$
and we call $K: M \rightarrow \mathbb{R}$ the \textit{Gaussian curvature}.
\end{corollary}

\begin{example}
    In dimension \( n = 2 \), Ricci curvature reduces to the classical \textit{Gauss curvature}, and can therefore be easily visualized.
\end{example}

One of the issues with working with the Riemannian curvature operator $R$ is that it contains a vast amount of information and is, as a result, sometimes overly complicated in nature for certain tasks. This is why curvature notions such as sectional curvature and Ricci curvature are used which extract certain curvature information from the Riemannian curvature itself.

For the next definition, note that if $f: X \rightarrow X$ is a linear map from a finitedimensional Euclidean vector space $X$ to itself, given any orthonormal basis $\left(e_{1}, \ldots, e_{n}\right)$, then 

$$
\operatorname{tr}(f)=\sum_{i=1}^{n}\left\langle f\left(e_{i}\right), e_{i}\right\rangle
$$
\section*{Undirected Graphs}
\noindent
A graph $G = (V,E)$ is defined as  pair of disjoint sets V, a set of \textit{vertices}, and E, a set of \textit{edges}. Consider a simple case where we define a graph as having 3 vertices such that we define the vertex set as $V(G) = \{v_1, v_2, v_3\}$ and let $v_1$ be connected to $v_2$ by a single edge and $v_2$ be connected to $v_3$ by a single edge. We can therefore define our edge set as $E(G) = \{\{v_1, v_2\}, \{v_2, v_3\}\}$. Then we can depict $G = (V,E)$ as done in Figure~\ref{fig:graph_example}.

\begin{figure}[ht]
    \centering
    \begin{tikzpicture}
        % Draw vertices
        \node[draw, circle, fill=black, inner sep=1.5pt, label=left:{$v_1$}] (v1) at (0, 1) {};
        \node[draw, circle, fill=black, inner sep=1.5pt, label=above:{$v_2$}] (v2) at (2, 2) {};
        \node[draw, circle, fill=black, inner sep=1.5pt, label=right:{$v_3$}] (v3) at (4, 1) {};
        % Draw edges
        \draw[thick] (v1) -- (v2);
        \draw[thick] (v2) -- (v3);
    \end{tikzpicture}
    \caption{A graph with three vertices and two edges.}
    \label{fig:graph_example}
\end{figure}

\noindent
We can also denote an edge connecting $v_1$ and $v_2$ as $v_1v_2$ or $(v_1, v_2)$. This is an example of an \textit{undirected} graph, in which the edge connecting $v_1$ and $v_2$ is not pointing in any one particular direction. Therefore, in this case edges $v_1v_2 = v_2v_1$ and the order does not matter. For every graph, each element $e \in E$ is a 2-element subset of V, so for all possible graphs we have $E \subseteq [V]^2$. By the fact that an edge can never be a vertex and vice versa, we always have $E \cap V = \emptyset $. Graphs are most often depicted visually for ease of reading, but note that there are unlimited correct ways to depict a single graph with regards to vertex location or edge style. However, the only information that matters is the exact edges and vertices present as determined by $v \in V$ and $e \in E$. Figure~\ref{fig:equal_graphs} shows that a single graph G can be drawn in a variety of correct ways. 
\begin{figure}[htbp]
    \centering
    \makebox[\textwidth]{\includegraphics[width=1\textwidth,keepaspectratio]{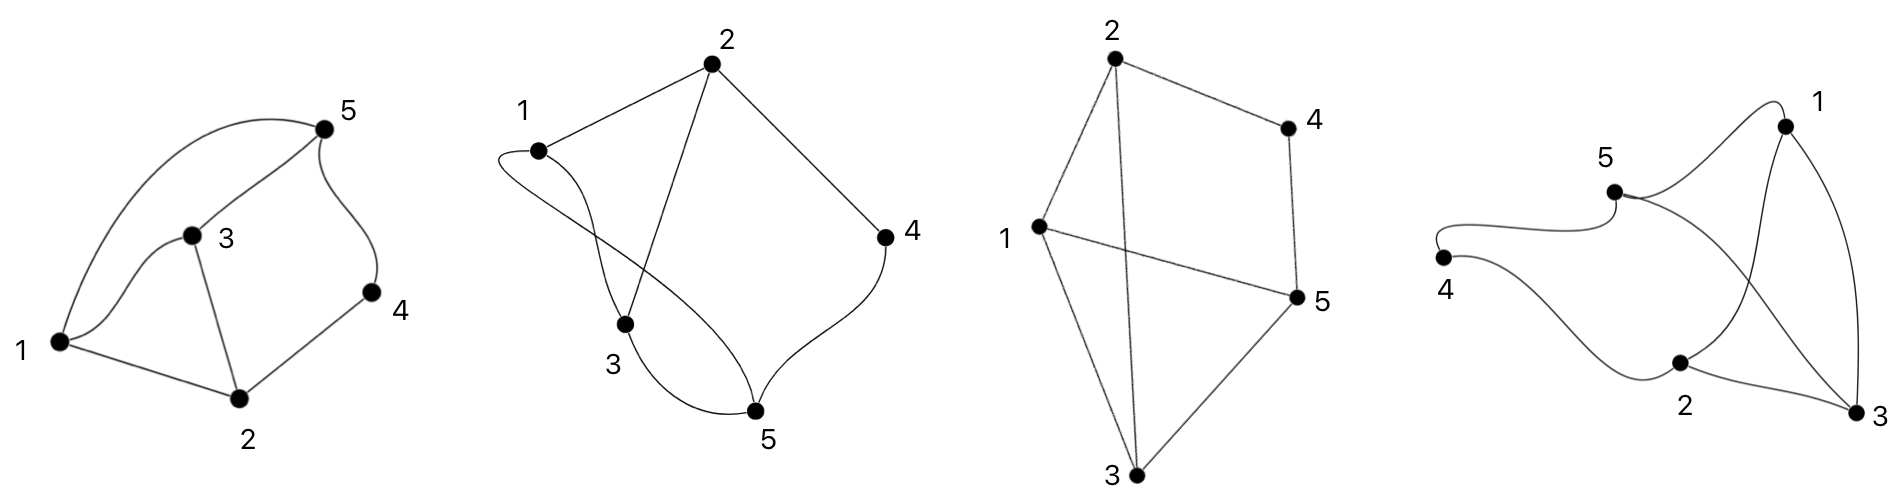}}
    \caption{Four equal representations of graph G.}
    \label{fig:equal_graphs}
\end{figure}

Consider this graph $G = (V,E)$ where $V(G) = \{1,2,3,4,5\}$ and
$$
E(G) = \{\{1,2\}, \{1,3\}, \{2,3\}, \{2,4\}, \{3,5\}, \{4,5\}, \{1,5\}\}
$$
as depicted in Figure~\ref{fig:equal_graphs}. Observe that $\{1,2\} \in E(G)$. By definition this means that vertices 1 and 2 are \textit{neighboring} vertices or \textit{adjacent} vertices. Furthermore, we say that the neighborhood $\mathcal{N}_x$ of a vertex $x$ is defined as the set of all neighboring vertices. For example, for G we have $\mathcal{N}_1 = \{2, 3, 5\}$ and $\mathcal{N}_3 = \{2, 4, 5\}$. Two edges are adjacent if they share a vertex. The \textit{degree} of any vertex $x \in V$ is defined as the number of edges connected to $x$, which can equivalently be defined as $\deg(x) = |\mathcal{N}_x|$. A graph is \textit{regular} if every vertex has the same degree, and \textit{$d$-regular} if every vertex has degree $d$. The \textit{order}, $|G|$ of a graph $G$ is equivalent to the number of vertices. Therefore $|V(G)| = |G|$. The \textit{size} of a graph $G$ is equal to the number of edges of $G$. Suppose that for any graph $G$ that $|G| = n$. Then we can equivalently refer to this graph as $G^n$. In this thesis, the graphs we work with will all be finite graphs. However, note that graph order can be infinite, such as the infinite $n \times n$ grid one can form all $n \in \mathbb{N}$. We call a graph \textit{empty} if it has no edges, though note it can have $|V(G)| \geq 0$. If $|V(G)| = 1$ and $G$ is empty such that we have a single point, we call this the \textit{trivial} graph. A graph is \textit{complete} if it is a simple, undirected graph where every pair of distinct vertices is connected by a single edge. For any graph $G$ comprised of sets $V$ and $E$, we can consider new graphs that can be formed by subsets of $V$ and $E$. For $G$ in Figure~\ref{fig:equal_graphs}, we can consider a new vertex set $V'(G) = \{1,2,3,5\}$ and $E'(G) = \{\{1,2\}, \{1,3\}, \{2,3\}, \{3,5\}, \{1,5\}\}$ where we remove vertex 4 and any of its edges such that $V'(G) \subset V(G)$ and $E'(G) \subset E(G)$. Then the new graph $G' \subset G$ that forms is called a \textit{subgraph} of $G$. There are a few different types of subgraphs. Consider a new subgraph $G'$ where for all $v \in V'(G)$, the edges that connect those vertices are all present in $E'(G)$. This is called an \textit{vertex-induced} (or just \textit{induced}) subgraph. Alternatively, consider the case where $V = V'$ but $E \subset E'$. We call this a \textit{spanning subgraph}. Up until this point, we have only discussed \textit{undirected} graphs which have edges that do not point in any particular direction. However, we can specify that an edge has a starting and ending node, which imposes directionality, making the graph a \textit{directed graph}. This will be discussed in extensive detail in Section 1.2. For now, assume that all graphs discussed are undirected. Until this point we have also only discussed simple graphs, but have not yet defined them. A \textit{simple graph} is a graph in which for any two vertices $x, y \in V(G)$, there are no repeated edges between $x$ and $y$ in the edge set. Additionally, for a graph to be simple there must be no edges $\{v,v\} \in E$, or in other words, no self-loops. It is not a requirement for all vertices to be connected to another vertex for a graph to be simple. Figure~\ref{fig:simple} shows visual representations of simple, non-simple, connected, and disconnected graphs.

\begin{figure}
    \centering

    \begin{minipage}{0.18\textwidth}
        \centering
        \begin{tikzpicture}[scale=0.7, every node/.style={circle, draw, fill=black, inner sep=1.5pt}]
            \node (a) at (0, 0) {};
            \node (b) at (-1, -1) {};
            \node (c) at (1, -1) {};
            \node (d) at (0, -2) {};
            \draw[thick] (a) -- (b);
            \draw[thick] (a) -- (c);
            \draw[thick] (b) -- (d);
            \draw[thick] (c) -- (d);
        \end{tikzpicture}
        \subcaption{}
    \end{minipage}
    \hfill
    \begin{minipage}{0.18\textwidth}
        \centering
        \begin{tikzpicture}[scale=0.7, every node/.style={circle, draw, fill=black, inner sep=1.5pt}]
            \node (a) at (0, 0) {};
            \node (b) at (-1, -1) {};
            \node (c) at (1, -1) {};
            \node (d) at (0, -2) {};
            \draw[thick] (a) -- (b);
            \draw[thick] (a) -- (c);
        \end{tikzpicture}
        \subcaption{}
    \end{minipage}
    \hfill
    \begin{minipage}{0.18\textwidth}
        \centering
        \begin{tikzpicture}[scale=0.7, every node/.style={circle, draw, fill=black, inner sep=1.5pt}]
            \node (e) at (0, 0) {};
            \node (f) at (-1, -1) {};
            \node (g) at (1, -1) {};
            \node (h) at (0, -2) {};
            \draw[thick] (e) -- (f);
            \draw[thick] (e) -- (g);
            \draw[thick] (f) -- (h);
            \draw[thick] (g) -- (h);
            \draw[thick, bend left] (e) to (g);
            \draw[thick, bend right] (e) to (g);
        \end{tikzpicture}
        \subcaption{}
    \end{minipage}
    \hfill
    \begin{minipage}{0.18\textwidth}
        \centering
        \begin{tikzpicture}[scale=0.7, every node/.style={circle, draw, fill=black, inner sep=1.5pt}]
            \node (i) at (0, 0) {};
            \node (j) at (-1, -1) {};
            \node (k) at (1, -1) {};
            \node (l) at (0, -2) {};
            \draw[thick] (i) -- (j);
            \draw[thick] (i) -- (k);
            \draw[thick] (j) -- (l);
            \draw[thick] (k) -- (l);
            \draw[thick] (i) to [out=30, in=60, loop] (i);
            \draw[thick] (k) to [out=300, in=330, loop] (k);
        \end{tikzpicture}
        \subcaption{}
    \end{minipage}
    \hfill
    \begin{minipage}{0.18\textwidth}
        \centering
        \begin{tikzpicture}[scale=0.7, every node/.style={circle, draw, fill=black, inner sep=1.5pt}]
            \node (m) at (0, 0) {};
            \node (n) at (-1, -1) {};
            \node (o) at (1, -1) {};
            \node (p) at (0, -2) {};
            \draw[thick] (m) -- (n);
            \draw[thick] (m) -- (o);
            \draw[thick] (m) to [out=30, in=60, loop] (m);
            \draw[thick] (o) to [out=300, in=330, loop] (o);
        \end{tikzpicture}
        \subcaption{}
    \end{minipage}

    \caption{Graphs varying in simplicity and connectivity: (a) simple and connected, (b) simple and disconnected, (c) non-simple by double-edge and connected, (d) non-simple by self-loops and connected, (e) non-simple and disconnected.}
    \label{fig:simple}
\end{figure}
A special type of simple graph  called a \textit{complete graph} is a graph where  every possible pair of vertices $u, v \in V$ is joined by a single edge $uv \in E$. A complete graph with $n$ vertices is denoted $K_n$, and the complete graphs $K_1$ through $K_9$ are depicted in Figure~\ref{fig:complete}

Suppose we have a graph G with two vertex classes or two subsets of $V(G)$ defined as $V_a, V_b \subset V(G)$ where $V_a \cap V_b = \emptyset$ $V_a \cup V_b  = V(G)$. Additionally, the only edges $e \in E (G)$ are edges that join vertices $v_{a(i)} \in V_a$ to $v_{a(j)} \in V_b$. Then we call $G$ a \textit{bipartite} graph. We can think of this as having a graph with two disjoint parts where all edges are connecting a vertex from one part to a vertex in the other part. This can be generalized for graphs with more than two vertex classes. We define a \textit{k-partite} graph as a graph with vertex classes \( V_1, V_2, \ldots, V_k \) where  \( V_i \cap V_j = \emptyset \) and \( V(G) = V_1 \cup V_2 \cup \cdots \cup V_k \) for \( 1 \leq i < j \leq k \), and with edge set $E$ that contains only edges that connect vertices of distinct vertex classes. 
\begin{figure}
    \centering
    \foreach \n in {1,2,3,4,5,6,7,8} {
        \begin{subfigure}{0.21\textwidth} % Scaled down from 0.3
            \centering
            \begin{tikzpicture}[scale=0.56, every node/.style={circle, draw, fill=black, inner sep=1.5pt}]
                \foreach \i in {1,...,\n} {
                    \node (\i) at ({360/\n * (\i - 1)}:1.5) {};
                }
                \foreach \i in {1,...,\n} {
                    \foreach \j in {\i,...,\n} {
                        \ifnum \i<\j
                            \draw[thick] (\i) -- (\j);
                        \fi
                    }
                }
            \end{tikzpicture}
            \caption{$K_{\n}$}
        \end{subfigure}
    }
    \caption{Complete graphs $K_n$ for $n = 1$ to $n = 8$.}
    \label{fig:complete}
\end{figure}
As one interprets a graph, it is natural to perhaps follow a path that you could take from one vertex to another if the vertices are not directly connected by an edge themselves. We formalize that concept here. A \textit{walk} $W$ on a graph is the sequences of vertices $v_1,v_2,..,v_n$ where all edges are defined as $v_i v_{i+1} \in E(G)$ for $1 \leq i \leq n$ where the vertices need not be distinct. If the vertices are distinct, the sequence of vertices is a path. A \textit{path} $P = (V,E)$ is a graph with $V(P) = \{v_1, v_2,...,v_k \}$ and $E(P) = \{v_1v_2, v_2v_3,...,v_{k-1}v_k \} $ is a graph such that all $v_i \in V(P)$ are distinct. Paths are denoted $P = v_1...v_k = v_k...v_1 $ or where $v_1$ and $v_k$ are the end vertices of the path which only have degree of 1. Consider for example a path within $K_6$ as depicted in Figure~\ref{fig:k6_variants}. We define this path as $P = 43165 = 56134$. The length of this path is equal to $|E(P)| = 4$, and therefore it is a $P^4$ path. Now, consider if the edge $\{4,5\}$ were in the edge set $E(P)$ forming a closed loop. This is called a cycle. A \textit{cycle} is defined as the non-empty graph $C:= v_{k-1}k_0 + P$ for a path $P = v_0v_2...v_{k-1}$. This is equivalent to saying that if $E(C)$ is the new edge set of a graph $C$, then if $E(C) = E(P) + v_{k-1}k_0$ then this graph is a cycle. We denote this cycle $C$ as $C = v_0v_2...v_{k-1}v0$ and define the length of the cycle as the number of edges, which will always be equivalent to its number of vertices unlike a path. Therefore, if $k$ is the length of a cycle such that $k = |V(C)| = |E(C)|$ then we call this a \textit{$k$-cycle}, or $C^k$.

A graph can be studied through eigenvalues and eigenvectors of a matrix that is associated with that graph. Spectral graph theory is a field that seeks to answer graphical questions using these eigenvectors and eigenvalues. In this section, we will discuss some of the essential definitions, theorems, and examples of spectral graph theory and then discuss relevant results and why matrix representations of graphs are particularly useful. We will discuss how the symmetry of undirected graphs allows spectral graph theory to be most useful, and will discuss how directed graphs can be studied using spectral graph theory given that they are not symmetric. We will denote an $i$-th row and $j$-th column entry in a matrix $M$ as $M(i,j)$. The $k$-th component of a vector $x$ will be denoted as $x(k)$. (To be continued)

\section*{Topological Spaces and Manifolds}
At  the foundation of Riemannian geometry is topology. To begin, we will begin by reviewing the fundamentals of topological spaces. We informally define a real n-dimensional \textit{manifold} as a topological space where the neighborhood around each point is locally Euclidean. We will define specific manifolds more formally in this section. First, we must review the general tools and definitions used to study manifolds more generally.

\begin{definition}
    A \textit{topology} on a nonempty set X is a collection $\mathcal{T}$ of subsets of $X$ such that: 
    \begin{enumerate}
        \item $X$ and $\emptyset$ belong to $\mathcal{T}$. 
        \item The union of any sets in $\mathcal{T}$ belongs to $\mathcal{T}$. 
        \item The finite intersection of any sets in $\mathcal{T}$ belongs to $\mathcal{T}$. 
    \end{enumerate}
And furthermore, we define a pair $(X, \mathcal{T})$ as a \textit{topological space}. Note that if $\mathcal{T}$ is known or understood by context, we will often refer to a topological space as just $X$.
\end{definition}

\noindent
\begin{definition}
    Let $\mathcal{M}$ be a topological space and let $U, V \subseteq \mathcal{M}$ be open sets. Then the homeomorphism $\varphi: U \rightarrow V$ where $\varphi(u) = (x_1(u),...,(x_n(u))$ is a \textit{coordinate system} on the set $U$, $x_1,...,x_n$ are the \textit{coordinate functions}. We can take the inverse $\varphi^{-1}$ and this is called the \textit{parametrization} of the set $U$. Furthermore if we let $\varphi_i^j = \varphi_j \circ \varphi_i^{-1}$. For any two charts $(U, \varphi)$ and $(V, \phi)$ where $U \cap V \neq \emptyset$ the  \textit{transition maps} are defined as: 
$$
\psi \circ \varphi^{-1}: \varphi(U \cap V) \to \psi(U \cap V)
$$
$$
\varphi \circ \psi^{-1}: \psi(U \cap V) \to \varphi(U \cap V)
$$

\end{definition}
\begin{example}
    Take for example 
\end{example}
\begin{definition}
     For the topological space $\mathcal{M}$, we define the pair $(U, \varphi)$ as a \textit{chart} on $\mathcal{M}$.  The collection of charts $\{U_\alpha, \varphi_\alpha\}$ where $U_\alpha$ cover $\mathcal{M}$ is called an \textit{atlas}. 
\end{definition}
\begin{definition}
    A topological space $X$ is \textit{first-countable} if it has a countable local basis at each point and is \textit{second-countable} if $X$ admits a countable basis. 
\end{definition}

\begin{definition}
    A topological space \( X \) is defined as \textit{connected} if there do not exist disjoint nonempty subsets \( U, V \subseteq X \) such that 
    \[
    X = U \sqcup V, \quad \overline{U} \cap V = \emptyset, \quad \overline{V} \cap U = \emptyset.
    \]
If a topological space is not connected then it is \textit{disconnected}.
\end{definition}

\begin{definition}
    A \textit{metric} $d$ on a topological space $X$ is a function $d: X \times X \rightarrow [0, \infty)$ such that for all $x,y,z \in X$, (1) $d(x,y) = 0$ \textit{i.f.f} $x = y$, (2) $d(x,y) = d(y,x)$, (3) $d(x,y) \geq 0$, (4)$d(x,y,z) \leq d(x,y) + d(y,z)$
    
\end{definition}

\begin{definition} 
    Let $(U, \varphi)$ be a topological space. 
    \begin{enumerate}
        \item U is a $T_0$\textit{-space} if for any two distinct point on U there is an open neighborhood of one point that does not contain the other.  
        \item U is a $T_1$\textit{-space} if each point of $U$ is a closed subset. 
        \item U is a \textit{Hausdorff space} or $T_2$\textit{-space}  if two distinct point on X always lie in disjoint open neighborhoods. 
    \end{enumerate}
\end{definition}

\begin{definition} A Hausdorff, second-countable topological space $\mathcal{M}$ is defined as an \textit{n-dimensional topological manifold} if it admits an atlas $U_\alpha, \varphi_\alpha \}$ for $\varphi_\alpha: U_\alpha \rightarrow \mathbb{R}^n$ for $n \in \mathbb{N}$. $\mathcal{M}$ is a \textit{smooth manifold} if all of its transition maps are $C^\infty$ diffeomorphisms. 
\end{definition}
\section*{Riemannian Metrics and Manifolds}
For the remainder of this chapter, when we discuss manifolds we will assume that they are connected topological manifolds, i.e. that they are Hausdorff and second-countable. Recall that for a point $x$ on a n-dimensional manifold $M$, the set of all tangent vectors at $x$ is the \textit{tangent space} at that point denoted as $T_xM$ where $T_xM$ is a vector space of dimension $n$.

\begin{definition}
    Let $M$ be a smooth manifold. \textit{A Riemannian metric} \( g \) on a \( M \) is a smoothly chosen inner product \( g_x : T_x M \times T_x M \to \mathbb{R} \) on each tangent space \( T_x M \) of \( M \). For each \( x \in M \), \( g = g_x \) we have:
\begin{enumerate}
    \item \( g(u,u) = 0 \) \textit{i.f.f.} \( u = 0 \).
    \item \( g(u,v) = g(v,u) \) for all \( u, v \in T_x M \)
    \item \( g(u,u) \geq 0 \) for all \( u \in T_x M \)
\end{enumerate}
Then we define $M$ as a \textit{Riemannian manifold}.
\end{definition}
Note: The metric \( g \) in this case is smooth because for smooth vector fields \( X \) and \( Y \), \( x \mapsto g_x(X_x, Y_x) \) is a smooth mapping.

\noindent
In other words, a Riemannian manifold $(M,g)$ is a $C^\infty$ manifold $M$ with a Euclidean inner product $g_x$ on all of the tangent spaces of the manifold where $g_x$ varies smoothly. If we consider two smooth vector fields $U$ and $V$, then the inner product $g_x(U,V)$ is a smooth function of $x$.

Remark: All tangent spaces $T_xM$ on $(M,g)$  are isometric to $\mathbb{R^n}$. This follows from the fact that all inner product spaces of equivalent dimension are isometric. 
\begin{definition}
Consider two Riemannian manifolds $(M,g)$ and $(X,h)$. A \textit{Riemannian isometry} between these manifolds is a diffeomorphism $\psi: M \rightarrow X$ such that $\varphi h  = g$
\begin{example}
    example of metric
\end{example}

\end{definition}
\section*{The Fundamental Theorem of Riemannian Geometry}
In this section we will prove the Fundamental Theorem of Riemannian Geometry that every Riemannian manifold has a unique Riemannian connection. To do this we will first review affine connections, torsion, and Riemannian connections. In order to do this, we will discuss directional derivatives on vector fields. 

\begin{definition}
Let X,Y be differentiable vector fields $\mathbb{R}^n \rightarrow \mathbb{R}^n$. At point $p$, the \textit{directional derivative} of $Y$ is: 
$$
(\nabla_X Y)(p) = \lim_{t \rightarrow 0}\frac{Y(p + tX(p)) - Y(p)}{t}
$$
where $\nabla_X Y$ itself forms a vector field $\mathbb{R}^n \rightarrow \mathbb{R}^n$.
\end{definition}
This follows from basic calculus where for a function $f: \mathbb{R}^n \rightarrow \mathbb{R}^m$ we define the directional derivative of a vector $v$ at a point $p$ as follows where $\nabla_v f(p)$ is a vector field $\mathbb{R}^n \rightarrow \mathbb{R}^m$ as:
$$
\nabla_v f(p) = \lim_{t \rightarrow 0}\frac{f(p + tv) - f(p)}{t}
$$

Observe that $\nabla$ is an operator that produces a single vector field $\nabla_X Y$ from inputted vector fields $X,Y$, as we have $\nabla(X,Y) = \nabla_X Y$.

\begin{theorem}
Let $\nabla: \mathfrak{X}\times \mathfrak{X} \rightarrow \mathfrak{X} $ where  $\mathfrak{X}$ denotes the space of all smooth vector fields from $\mathbb{R}^n$ to $\mathbb{R}^n$, where $X,Y,Z \in \mathfrak{X}$. Let $\nabla$ be the operator from Definition 2.1.15. Also let $f,g$ be defined as differentiable function from $\mathbb{R}^n$ to $\mathbb{R}^n$. Then the properties below hold: 
\begin{enumerate}
    \item $\nabla(fX + gY, Z) = f\nabla(X, Z) + g\nabla(Y, Z)$
    
    \item $ \nabla(X, Y + Z) = \nabla(X, Y) + \nabla(Y, Z) $
    \item $\nabla(X, fY) = f\nabla(X, Y) + (Xf)Y$
\end{enumerate}
\end{theorem} 

Our ultimate goal is to define directional derivatives on a manifold $M$ with an operator analogous $\nabla$. Definition 2.1.15 takes advantage of that fact that we are working with Euclidean space and that  $\mathbb{R}^n$ is \textit{affine}, which means that vectors can be added to points to get new points. Consider instead an arbitrary manifold $M$ that need not be embedded in Euclidean space. A directional derivative of a smooth function $f$  in the derivation of $X_p \in T_pM$ can be defined as
$$
\nabla_{X_p}f = X_p f
$$
There is no canonical basis for $T_p M$ and so there is not a canonical way for defining the directional derivative of vector field $Y$  when working with any arbitrary manifold, unlike the simple case of $\mathbb{R}^n$. This is because if we wanted to add a vector from $T_p M$ to $p$ on a manifold, we will find that this is not well-defined. Addition of vectors from distinct tangent spaces of a manifold is also not well-defined either. To resolve this issue, we can define a directional derivative operator on manifolds by taking advantage of properties of Theorem 2.1.16. 
\begin{definition} \cite{TuLoringW2017DG:C}
    Let $M$ be a smooth manifold where $X,Y,Z \in \mathfrak{X}$ and $f,g$ be defined as differentiable functions on $M$. Let \( \mathcal{F} \) be the ring \( C^\infty(M) \) of \( C^\infty \) functions on \( M \). Then the $\mathbb{R}$-bilinear map
    $\nabla: \mathfrak{X}(M) \times \mathfrak{X}(M) \rightarrow \mathfrak{X}(M) $ is an \textit{affine connection} if the following are satisfied for all \( X, Y \in \mathfrak{X}(M) \):
\begin{enumerate}
    \item \( \nabla_X Y \) is \( \mathcal{F} \)-linear in \( X \),
    \item For \( f \in \mathcal{F} \),
    \[
    \nabla_X (fY) = (Xf) Y + f \nabla_X Y
    \] (\( \nabla_X Y \) satisfies the Leibniz rule in \( Y\))
\end{enumerate}

\end{definition}
\begin{example}
    Example of affine connections
\end{example}

In physics, the term \textit{torsion} is used to refer to a force that twists an object in some way. In Riemannian geometry, conceptually torsion can be thought of as the extent to which a connection fails to be symmetric. In this sense, it is able to capture the extent to which basis vectors are "twisted" around a point during parallel transport. We will discuss this more formally and then return to this conceptual idea. 

\begin{definition}
    The \textit{torsion $T$} or \textit{torsion tensor} of a connection $\nabla$ is defined as: 
$$
T(X,Y) = \nabla_X (Y) - \nabla_Y (X) - [X,Y]
$$
and a connection is called \textit{torsion-free} if $T(X,Y) = 0$ for all $X,Y \in \mathfrak{X}(M)$
\end{definition}

\begin{theorem} (The Fundamental Theorem of Riemannian Geometry) \cite{PetersenPeter2006Rg}
Let $X \rightarrow \nabla X$ be an assignment on $\mathbb{R}^n$. The assignment is uniquely defined by the following: 
\begin{enumerate}
\item $\nabla X$ is a $(1,1)$\textit{-tensor}
$$
\nabla_{\alpha v + \beta w}X = \alpha \nabla_v X + \beta \nabla_w X
$$
\item $X \rightarrow \nabla X$ is \textit{torsion-free}
$$
\nabla_X Y - \nabla_Y X = [X,Y]
$$
\item  $X \rightarrow \nabla X$ is a metric 
$$
d(g(X,Y)) = g(\nabla X, Y) + g(X, \nabla Y)
$$
where g is canonical metric on $\mathbb{R}^n$
\item For functions $f: \mathbb{R}^n \rightarrow \mathbb{R}$, $X \rightarrow \nabla X$ is a derivation 
\begin{align*}
\nabla(X + Y) = \nabla X + \nabla Y, \\
\nabla (fX) = d(f)X + f \nabla X
\end{align*}
\end{enumerate}
In other words, there is a unique Riemannian connection for any Riemannian manifold $M$.

\section*{Classical Results on Directed Graphs}

\begin{definition} Let $D = (V,A)$ be a digraph. A \textit{Hamiltonian path} or \textit{Hamilton path} of $D$ is defined as path of $D$ which contains every vertex of $D$. In this thesis we will denote this type of path as $P_H$, and $P_H(D)$ to be a Hamiltonian path of $D$. If the the vertex set of $D$ is $V = \{v_1,v_2,...,v_k\}$ then a $P_H$ path of $D$ is a path which contains all $v \in V$ only once. 
\end{definition}
\begin{theorem}
\textbf{R\'edei's Theorem} \cite{Redei1934} Every tournament contains an odd number
of Hamiltonian dipaths.
\end{theorem}
In order to prove Theorem 1.2.5, we will first introduce the following Lemma.
\begin{lemma} (Inclusion Exclusion, \cite{bang-jensen_classes_2018} Lemma 2.6.2) 
Let \( Z \) be a finite set, and consider a function \( f: 2^Z \to \mathbb{N} \) that assigns real values to subsets of \( Z \). Define also a function \( g: 2^Z \to \mathbb{N} \) by summing over all supersets of a given set:

\[
g(X) = \sum_{\{ Y \mid X \subseteq Y \subseteq Z \}} f(Y).
\]

Then, the function \( f(X) \) can be defined as

\[
f(X) = \sum_{\{ Y \mid X \subseteq Y \subseteq Z \}} (-1)^{|Y|-|X|} g(Y).
\]
\end{lemma}
\begin{proof}
We apply the Binomial Theorem. Observe that

\[
\sum_{\{ Y \mid X \subseteq Y \subseteq W \}} (-1)^{|Y|-|X|}
\]

can be rewritten as a sum over binomial coefficients:

\[
\sum_{k=|X|}^{|W|} \binom{|W| - |X|}{k - |X|} (-1)^{k - |X|}.
\]

By the Binomial Theorem,

\[
\sum_{k=0}^{m} \binom{m}{k} (-1)^k = (1 - 1)^m,
\]
and therefore, 
\[
\sum_{k=|X|}^{|W|} \binom{|W| - |X|}{k - |X|} (-1)^{k - |X|} = (1-1)^{|W| - |X|}
\]

Let $X \subset W$. Then $|X| < |W|$ and therefore $ |W | - |X| = n$  for some $n \in \mathbb{N}$ and we get: 
\[
\sum_{k=|X|}^{|W|} \binom{|W| - |X|}{k - |X|} (-1)^{k - |X|} = (0)^n = 0
\]
Let \( X = W \), then $ |W | - |X| = 0 $ and we get: 
\[
\sum_{k=|X|}^{|W|} \binom{|W| - |X|}{k - |X|} (-1)^{k - |X|} = (0)^0 = 1
\]
It follows that,
\[
f(X) = \sum_{\{ W \mid X \subseteq W \subseteq Z \}} f(W) \sum_{\{ Y \mid X \subseteq Y \subseteq W \}} (-1)^{|Y|-|X|}.
\]

Since the first sum evaluates to 1 if \( W = X \) and 0 otherwise, we can swap the order of summation:

\[
f(X) = \sum_{\{ Y \mid X \subseteq Y \subseteq Z \}} (-1)^{|Y|-|X|} \sum_{\{ W \mid Y \subseteq W \subseteq Z \}} f(W).
\]

Observe that: 
$$
 \sum_{\{ W \mid Y \subseteq W \subseteq Z \}} f(W) = g(Y)
$$
Therefore, 
\[
f(X) = \sum_{\{ Y \mid X \subseteq Y \subseteq Z \}} (-1)^{|Y|-|X|} g(Y).
\]
And the proof is complete. 
\end{proof}
We will now apply the Inclusion-Exclusion principle to prove R\'edei's Theorem following \cite{bang-jensen_classes_2018,graham1995handbook}.
\begin{proof}
Let $D = (V,A)$ be a \textit{tournament} with $V(D) = \{1,2,\dots,k\}$. Let the set of all Hamiltonian paths be $P_H(D)$, $|P_H(D)|$  the number of Hamiltonian paths of $D$,  $h \in P_H(D)$ be a Hamiltonian path in $D$, and $H \subseteq P_H(D)$ be a subset of Hamiltonian paths of $D$. Recall that we can permute the vertex set of $D$. Let $\mathcal{S}_k$ be the set of all permutations on $V$. Let $A_i$ be a subset of the arc set $A$. Furthermore, for all $\pi \in \mathcal{S}_k$, we define the subset $A_\pi$ of $A(D)$ as:
\[
A_\pi = \{(\pi(i),\pi(i + 1)) \mid 1 \leq i \leq k-1\} \cap A.
\]
When paired with $V(D)$, induces a subdigraph of $D$. Every component of this subdigraph is a directed path. For all $A_i \subseteq A$, we define  $g(A_i)$ as the number of permutations  $\pi$ of vertex set such that $A_i$ is a subset of $A$ and define $f(A_i)$ as the number of permutations  $\pi$ of vertex set such that $A_i$ is a subset of $A$:
\[
g(A_i) := |\{\pi \in \mathcal{S}_k \mid A_i \subseteq A_\pi\}|,
\]
\[
f(A_i) := |\{\pi \in \mathcal{S}_k \mid A_i = A_\pi\}|.
\]
And therefore we have the following relation,
$$
g(A_i) = \sum_{A_i \subseteq A_j \subseteq A} f(A_j)
$$

By the Inclusion–Exclusion Principle from Lemma 1.2.6,
\[
f(A_i) = \sum_{A_i \subseteq A_j \subseteq A} (-1)^{|A_j| - |A_i|} g(A_j).
\]
We obtain $g(A_j) = n!$ if and only if the spanning subdigraph with edge set $A_j$ is a disjoint union of $n$ directed paths. Therefore it follows that $g(A_j)$ is odd if and only if $A_j$ induces a Hamiltonian directed path of $D$. We define $h(A_i)$ as the number of Hamiltonian paths of $A_i$ as follows:
\[
h(A_i) := |\{h \in P_H(D) \mid A_i \subseteq A(h) \}|,
\]
we can rewrite $f(A_i)$ as
\[
f(A_i) = \sum_{\{h \in P_H(D) \mid A_i \subseteq A(H)\}} (-1)^{k-1-|A_i|} \equiv h(A_i) \pmod{2}.
\]
A transitive tournament $T_k$ has a unique Hamiltonian path, and therefore we in the transitive case we know that this theorem holds. Any tournament $T$ on $k$ vertices can be derived from the transitive tournament $T_k$ by reversal of selected arcs. Thus we will show that the number of Hamiltonian dipaths is invariant under the reorientation of any single arc $a \in A$. Taking $A_i = \{a\}$ in the above formulation, we have:
\[
f(a) \equiv h(a) \pmod{2}.
\]
Suppose we obtain some tournament $T'$ from $T^k$ by reorienting some $a$, then:
\[
h(T') = h(T) + f(a) - h(a) \equiv h(T) \pmod{2}.
\]
and we are done.
\end{proof}
\begin{definition} Let $D = (V,A)$ be a digraph. Then, 
\begin{enumerate}
    \item \textit{Non-arcs} of $D$ are the elements $ (u,v) \in (V \times V) \ A$. These are the vertex pairs $(u,v) \in V \times V$ where $(u,v) \notin A$. 
    \item $D^{rev} = (V, A^{rev})$ is the digraph where the arc set is defined as $A^{rev} = \{(u,v) \mid (v,u) \}$ where all edges are reversed. $D^{rev}$ is the \textit{reversal} digraph of $D$. 
    \item $\overline{D} = (V, \overline{A})$ is the digraph where the arc set is defined as $\overline{A} = (V \times V) \ A$. This is called the \textit{complement} of $D$ and is the digraph formed by removing all arcs of $D$ and adding all non-arcs to the arc set. 
\end{enumerate}
\begin{theorem}
\textbf{Camion-Moon Theorem} \cite{CAMIONP1959CECH}, \cite{MoonJohnWToT} Every strongly connected tournament has
a Hamilton dicycle.
\end{theorem}

\begin{theorem}
    \textbf{Gallai–Milgram Theorem} Let $D$ be a digraph containing no loops. Then there exists a path cover $\mathcal{P}$ of $D$ and an independent set of vertices $S = \{v_P \mid P \in \mathcal{P})$ such that for all $P \in \mathcal{P}$, $v_P \in P$. 
\end{theorem}
Before we begin proving the above theorem, we discuss a few definitions and conventions: 
\begin{itemize}
    \item A \textit{path cover} $\mathcal{P} = \{P_1, P_2,...,Pn\}$ is defined as a finite set of disjoint paths $P$ of $D$ which over all vertices of the graph such that each $v \in V(D)$ belongs to only one path $P$. See Figure X for a path cover $P$.  
    \item Every \textit{dipath} has an initial and terminal vertex, also called start and end vertices. We define $T(\mathcal{P})$ as the set of all terminal vertices for paths $P \in \mathcal{P}$. It is easy to see that we will always have $|T(\mathcal{P})| = |\mathcal{P}|. $
    \item Suppose we are discussing the composition of a path $P_i$ and let $v \in V(D)$. Then $P_i + v$ is a new path with $v$ as the new end vertex.
    \item Let $\mathcal{P}_i$ and $\mathcal{P}_j$ be any two distinct path covers of a digraph $D$ for $i \neq j$.  We say that a path cover $\mathcal{P}_i$ is \textit{T-minimal}  if no $T(\mathcal{P}_j)$ forms a proper subset of $T(\mathcal{P}_i)$. 
\end{itemize}
\vspace{0.2cm}
\begin{example} (Path covers). Suppose we have digraph $D$ defined such that $V(D) = \{v_1,v_2,..,v_6\}$ and $A(D) = \{v_1v_3, v_3v_4, v_4v_5, v_6v_5, v_6v_3, v_6v_2, v_2v_1\}$ as depicted in Figure 1.10. Then example path covers $\mathcal{P}$ of $D$ and $\mathcal{Q}$ of $D$ are: 
\begin{align*}
    \mathcal{P}(D) &= \{P_1 = v_6v_3v_4v_5,  P_2 = v_2v_1\}\\
    \mathcal{Q}(D) &= \{P_3 = v_1v_3v_4v_5,  P_4 = v_6v_2\}\\
    \mathcal{R}(D) &= \{P_5 = v_6v_2v_1v_3v_4v_5\}\\
    \mathcal{S}(D) &= \{P_2 = v_2v_1,  P_6 = v_6v_3, P_7 = v_4v_5\}
\end{align*}
Furthermore, we define the set of terminal vertices for each path covering as follows: 
\begin{align*}
    T(\mathcal{P}) &= \{v_1, v_5\},  T(\mathcal{Q}) = \{v_5, v_2\}, 
    T(\mathcal{R}) = \{v_5\},  T(\mathcal{S}) = \{v_1, v_5, v_3\}
\end{align*}
And it follows that only path cover $\mathcal{R}$ is \textit{T-minimal}.
\end{example}
\begin{proof} (Following \cite{diestel_graph_2017} Thm. 2.5.1, \cite{GrinbergDarij2023Aitg} Thm. 10.2.6) 
It is obvious that there always exists a path cover for $D$. For example, for every $D$ we can construct a path cover in which all paths are singular arcs. Such paths are called trivial paths. We will prove by induction on $|D| = n$ that for all path covers $\mathcal{P}$ of $D$ with minimal $|\mathcal{P}|$, that the set $S$ exists. It is equivalent to prove by induction on $|D|$ that for all path covers $\mathcal{P}$ of $D$ with minimal $T(\mathcal{P})$, that the set $S$ exists. Let $T(\mathcal{P})$ be independent where $T(\mathcal{P}) = \{v_1,,..., v_{k-1}, v_k\}$. Then we are done because then the independent set $S$ exists. If $T(\mathcal{P})$ is independent it means that for all $v_i,v_j \in T(P)$, $\overrightarrow{v_iv_j} \notin A(D)$. Recall that $v_i \in T(\mathcal{P})$ refers to the terminal vertex of path $P_i \in \mathcal{P}$. Without loss of generality, suppose that $T(\mathcal{P})$ is not independent such that there is an arc connecting two distinct terminal vertices $v_i, v_j$ on distinct paths. Without loss of generality suppose that $i = k-1$, $j = k$.

Therefore suppose that we construct a new arc $\overrightarrow{v_k v_{k-1}} \in A(D)$ between terminal vertices of $P_k$ and $P_{k-1}$. We now have an extended path of the original $P_{k-1}$, which we now call $P_{k-1} + v_k$. However, given that we are considering only path covers with minimal $T(\mathcal{P})$, it follows that $P_{k-1}$ contains other vertices besides its terminal vertex $v_k$. Let $v \in P_{k-1}$ denote the vertex prior to the terminal vertex $v_{k-1}$ (such that $\overrightarrow{vv_{k-1}}$ is an arc in $P_{k-1}$). Consider the new digraph defined as $D' := D \setminus v_{k-1}$, where $v_{k-1}$ is removed along with all arcs containing $v_{k-1}$ such that $|D| = n -1$. The path $P_{k-1}'$ now has end vertex $v$ and does not contain $v_{k-1}$. There is a path cover of $D'$ defined as:
\[
\mathcal{P'} := \{P_1, \dots, P_{k-1}', P_k\}.
\]
We apply our induction hypothesis to $\mathcal{P'}$. We define $T(\mathcal{P}')$:
\[
T(\mathcal{P}') := \{v_1, v_2, \dots, v, v_k\}.
\]
Recall that we are trying to show that for $D$ there exists a path cover $\mathcal{P}$ and an independent set of vertices $S \subseteq V(D)$ such that $S$ contains one vertex exactly from each $P \in \mathcal{P}$. Therefore we are done if we find such a set $S$ for the path cover $\mathcal{P}'$ because such an independent set $S$ would also work for $\mathcal{P}$ as it would also contain exactly one vertex from each path $P \in \mathcal{P}$. It suffices to show by our induction hypothesis that $\mathcal{P}'$ is $T$-minimal, as this would apply the existence of $S$ for both $\mathcal{P}'$ and subsequently $\mathcal{P}$.

Suppose that $\mathcal{P}$ is T-minimal. Suppose for the sake of contradiction that $\mathcal{P}'$ is not T-minimal and $D'$ has a path cover $\mathcal{R'}$ such that $T(\mathcal{R'})$ is a proper subset of $T(\mathcal{P}')$ such that $T(\mathcal{R'}) \subset T(\mathcal{P}')$ and $T(\mathcal{R'}) \neq (\mathcal{P}')$. This implies:
$$
|T(\mathcal{R'})| < |T(\mathcal{P'})| = k
$$
We will now evaluate the following cases: $(1)$ $v \in T(\mathcal{R'})$, $(2)$ $v_k \in T(\mathcal{R'})$ and $v \notin T(\mathcal{R'})$, $(3)$ $v_k \notin T(\mathcal{R'})$ and $v \notin T(\mathcal{R'})$.

For case $(1)$, suppose for the sake of contradiction that $v \in T(\mathcal{R'})$. Then for the path $P \in \mathcal{R'}$ that contains $v$ as its terminal vertex, we can add the vertex $v_{k-1}$ such that this path is now defined as $P = \{v_1,...,v,v_{k-1}, v_k\}$. Then we get a new path cover $\mathcal{R}$ of $D$ such that $T(\mathcal{R}) \subseteq T(\mathcal{P})$. This is a contradiction because then $\mathcal{P}$ is not $T$-minimal. For case $(2)$, suppose for the sake of contradiction that $v_k \in T(\mathcal{R'})$ and $v \notin T(\mathcal{R'})$. It follows that $T(\mathcal{R'}) \subseteq \{v_1,..,v_{k-2}, v_k\}$ and there exists a path $P \in \mathcal{R'}$ such that $T(P) = v_k$ which we will call $P_k$. Let us construct a new arc such that $P_k + v_{k-1}$ and replace this with the original $P_k$ in $\mathcal{R'}$ to obtain a new path cover $\mathcal{R}$ of $D$ containing $P_k + v_{k-1}$ such that $T(\mathcal{R}) \neq T(\mathcal{P})$ but $T(\mathcal{R}) \subseteq T(\mathcal{P})$. However, then we have a contradiction for case $(2)$ because this would imply that $\mathcal{P}$ is not $T$-minimal. Lastly consider case (3) and suppose for the sake of contradiction that $v_k, v \notin T(\mathcal{R'})$. Then we have that $T(\mathcal{R'}) \subseteq \{v_1,...,v_{k-3}, v_{k-2}\}$ such that $|T(\mathcal{R'})|\leq k-2$. Again we will construct an arc $v_{k-2}$ to $v_{k-1}$ such that we obtain a new path cover $\mathcal{R}$ of $D$ such that $T(\mathcal{R}) \neq T(\mathcal{P})$ but $T(\mathcal{R}) \subseteq T(\mathcal{P})$. Again we have a contradiction because $\mathcal{P}$ is $T$-minimal.

Since all three cases present contradictions, we have shown that $\mathcal{P'}$ is T-minimal. We can then apply induction hypothesis to $D'$ rather than $D$. It follows then that path cover $\mathcal{P'}$ of $D$ has an independent set of vertices $S = \{v_P \mid P \in \mathcal{P}')$ such that for all $P \in \mathcal{P}'$, $v_P \in P$. We showed that this set $S$ is also  an independent set of vertices $S = \{v_P \mid P \in \mathcal{P})$ such that for all $P \in \mathcal{P}$, $v_P \in P$. Therefore, we have proved the Gallai-Milgram theorem. 
\end{proof}
\end{definition}

\end{theorem}
\newpage \ \newpage
